# Supplementary material for: Knowledge of Pretrained Language Models on Surface Information of Tokens
Source: arXiv:2402.09808 source file (2024-02-22)
Supplement: Supplementary file 1 [file 99_appendix.tex]

\appendix
\section{Details of Target PLMs}

% モデルごとのembedding sizeも書いたほうが良い

% word2vec
%分散表現のパラメータ数は768，学習エポック数は10，学習対象にする単語の最小出現回数は10とした．
%また，学習に用いる窓幅は5とした．

\section{Training of MLP}
% MLPのspecと学習方法，選択方法を書く？
In all experiments, we used three-layered MLPs and the size of hidden parameters were 2,096.
We trained the MLP with the loss functions explained in each section with 10 training eporhs.
The batch size was 512.
This number of training steps is enough to obtain the model whose loss values are converged.
During the training of MLPs, the input embeddings of subwords or words are frozen to save the knowledge acquired in the pretraining.
All experiments were conducted on NVIDIA RTX A6000.

\section{Length Prediction by LLaMA2}
% llamaのMSEものせる

%\section{Word2Vec, FastText, GloVe\\の詳細}
%\label{sec:model_construction_w2v}
%分析で用いるWord2VecとFastTextのモデルは，Gensim~\cite{rehurek2011gensim}が提供するパッケージを用いて独自に学習を行った．
%どちらも，英語のWikipediaから作成した20GBのテキストを学習データとして用い，Skip Gramによる学習を行った．
%学習データは，NLTK~\cite{bird2006nltk}の英語用トークナイザーによって句読点等の分割を行ってから利用した．
%分散表現のパラメータ数は768，学習エポック数は10，学習対象にする単語の最小出現回数は10とした．
%また，学習に用いる窓幅は5とした．
%GloVeのモデルには，glove-wiki-gigaword-300を使用した．

%\section{モデルごとの入力例}
%\label{sec:input_token}
%単語単位の検証においては，学習済みの言語モデルで単語を構成するサブワード列をエンコードした結果を分散表現として用いる．
%この時，特定の入力トークンに対応する出力を，単語全体の分散表現として利用する．
%事前学習済みの言語モデルの構造や，対応している特殊トークンに応じて，どの入力トークンに対応する出力を用いるかは異なる．
%表\ref{tbl:input_example}に，モデルごとに対応する入力トークンをまとめた．
%表において，下線で示したトークンに対応する出力を，単語の分散表現として各検証で学習するMLPに入力する．
%BERTとCANINEの各モデルについては，先頭に挿入される特殊トークンに対応する出力を，単語の分散表現として用いた．
%T5では，文の末尾に追加される特殊トークンに対応する出力を単語の分散表現として用いた．
%LLaMA2の各モデルでは，入力の末尾のトークンに対応する出力を単語の分散表現として用いた\footnote{LLaMA2は単方向の言語モデルであり，入力内容によらず1トークン目に対応する出力結果は一定であるため，先頭の特殊トークンを用いることはできない．}．

%\input{tables/input_example}

%\section{文字数の詳細な予測結果}
%図\ref{fig:bert-length-word-box}と図\ref{fig:llama-length-word-box}に，それぞれBERT-base-casedとLLaMA2-7B-chatを用いた単語単位での文字数予測（\S \ref{sec:length-explanation}，表\ref{tbl:main_result}）と正解の文字数との比較結果を示した．
%横軸は正解の文字数，縦軸は回帰モデルが予測した文字数であり，赤い直線は正解を示す．
%結果より，どちらのモデルを用いた場合であっても，3から10文字程度の長さの単語であれば，それなりに正解に近い文字数を予測できていると言える．
%特にLLaMA2のモデルは，比較的長い単語であっても予測が大きく外れることが無く，表層的な長さの知識をある程度の範囲で獲得できていると言える．

\begin{figure}[t]
    \centering
    \includegraphics[width=7.8cm]{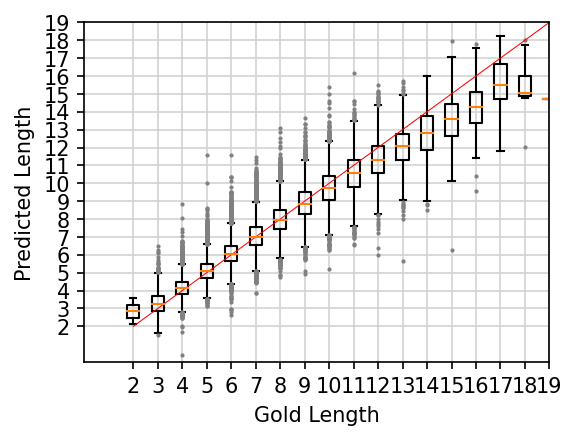}
    \caption{
        Comparison of the predicted length and the gold length of word-level inputs with LLaMA2-7B-chat.
        The red line indicates the correct prediction.    }
    \label{fig:llama-length-word-box}
\end{figure}
